# Supplementary material for: [Dissertation] Fundamental Limits to Single-Photon Detection
Source: arXiv:2210.04089 source file (2022-10-08)
Supplement: Supplementary file 1 [file appendix1.tex]

\chapter{Appendix}
